# Supplementary material for: Lesion-based Contrastive Learning for Diabetic Retinopathy Grading from Fundus Images
Source: arXiv:2107.08274 source file (2021-07-17)
Supplement: Supplementary file 1 [file appendix.pdf]

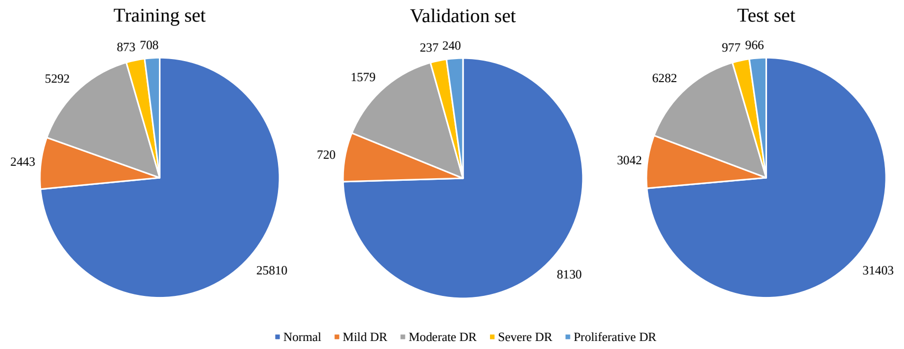


**Fig. A1.** The class distribution of EyePACS.

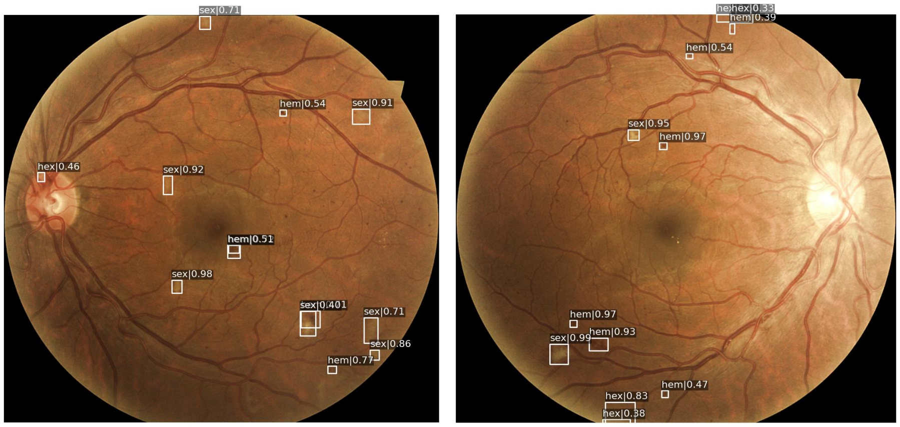


**Fig. A2.** Representative lesion detection results. Prediction classes hem, sex, and hex respectively denote hemorrhage, soft exudate, and hard exudate. The number attached to each bounding box represents the confidence score.

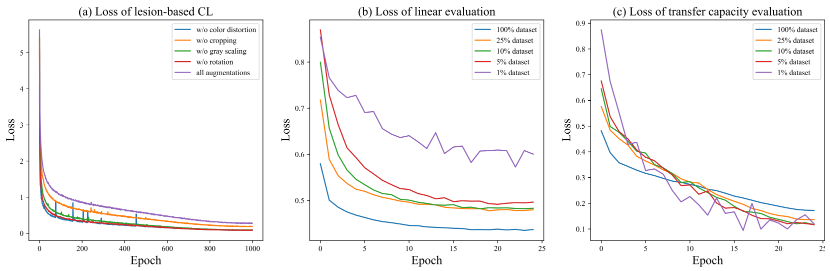


**Fig. A3.** Training curves of the proposed lesion-based CL under a detection confidence threshold of 0.8. (a) is the training loss curve of our contrastive prediction task. (b) and (c) are the training loss curves of linear evaluation and transfer capacity evaluation.

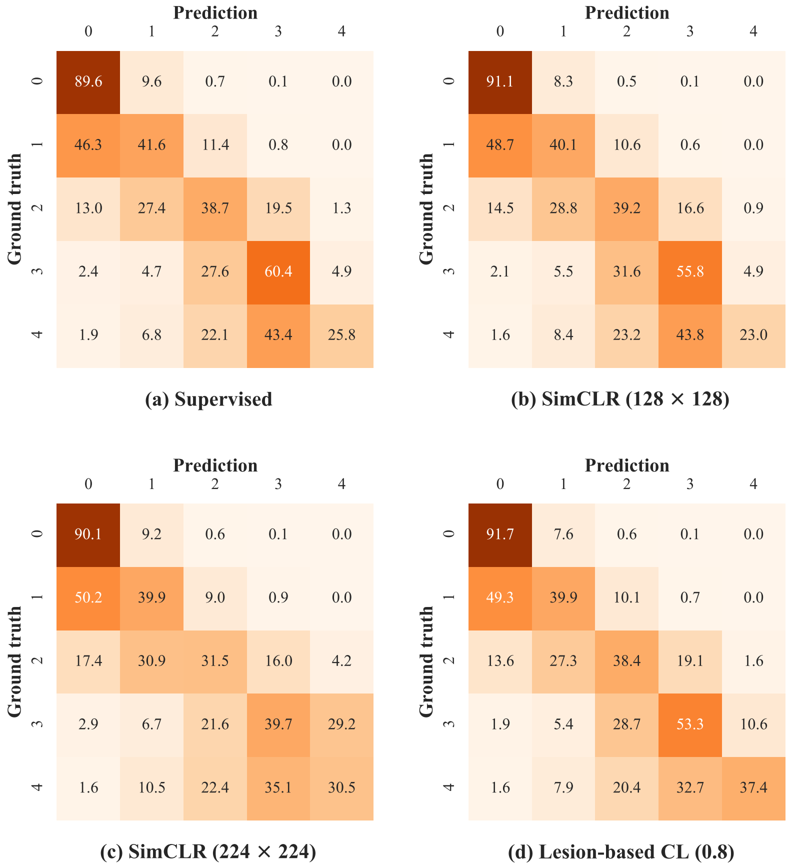


**Fig. A4.** Confusion matrices from transfer capacity evaluation of different methods on the 25% partial dataset. Our lesion-based CL is based on patches obtained from a detection network with a confidence threshold of 0.8.
